# Supplementary material for: Unexpected Benefits of Self-Modeling in Neural Systems
Source: arXiv:2407.10188 source file (2024-07-23)
Supplement: Supplementary file 2 [file appendix.tex]

\appendix
\section{Appendix}
\subsection{MNIST Variants}

We explored using deeper networks for MNIST as well. The extreme overparameterization of these large networks relative to the simplicity of the classification task presented an interesting test bed for demonstrating self-modeling's ability to reduce effective model complexity. Figure \ref{fig:vary_target_layer} shows the
results. When the earliest, largest layer was targeted (layer 0), self-modeling had the largest beneficial
effect. The RLCT attained its lowest value, significantly below baseline. The gap between train and test
loss was at its minimum, and the test loss was significantly lower than the baseline. The self-modeling variant used fewer effective parameters, and this resulted in better generalization and in fact overall out-of-distribution performance. As the targeted layer
was changed, the benefit of self-modeling diminished. When layer 1 was targeted, the benefits were
reduced; when the third, fourth, or fifth layers were targeted, no significant benefits were observed. The factor that determined whether self-
modeling was beneficial may have been the size of the target layer, the position of the target layer within
the larger architecture, or an interaction between the two.

\begin{figure}[h!]
    \centering
    \includegraphics[width=\linewidth]{other_figures/vary_target_layer_with_loss_with_baseline.png}
    \caption{Targeting early layers in this architecture provides the greatest benefit to RLCT and generalization.}
    \label{fig:vary_target_layer}
\end{figure}

\subsubsection{Vary Target Layer Size}

In the previous set of experiments, we varied the location and size of the target layer. To isolate the effect of one, we fix the second layer as the target and vary its size. Specifically, the hidden layer structure is $[2000, X, 500, 250, 100, 20]$ where $X$ varies between $5000$ and $500$. Now we repeat each baseline measurement to ensure that the architecture itself is not responsible for any new effects. We see a relatively flat trend in RLCT across an order of magnitude of test layer widths. On the other hand, when the target layer is very large, the generalization error is minimized. The baseline architecture with the largest second layer does not see a small generalization gap. This points again to a relationship between self-modeling large layers and improved generalization. 

\begin{figure}[h!]
    \centering
    \includegraphics[width=\linewidth]{other_figures/vary_target_layer_width_with_loss_with_baseline.png}
    \caption{When the size of the target layer is large, we see the smallest generalization error.}
    \label{fig:vary_target_layer_width}
\end{figure}

\subsubsection{Vary Target Layer Position}

A natural next step is to vary position while keeping size of the target layer fixed. In order to accomplish this, network is composed of uniform layers each $1000$ neurons in width. In this experiment, we did not see much of an effect on generalization or performance. The RLCT did change with target layer but there is no discernible trend and the large variance of the measurement renders it unclear whether or not position of target layer matters when the network is uniform in width. 

\begin{figure}[h!]
    \centering
    \includegraphics[width=\linewidth]{other_figures/fixed_width_with_loss_with_baseline.png}
    \caption{Varying the target layer in a network with fixed width layers.}
    \label{fig:fixed_width}
\end{figure}

\subsubsection{Vary Surrounding Layer Size}

Inspired by the ideas of (???) Next we investigate fixing the target layer and size while the two layers immediately before and after the target have their size varied. Hidden layers are given by $[X, 1000, X, 500, 20]$ where $X$ takes values between $2000$ and $100$. We see a linear decrease in RLCT, but when compared to the same slope of the baseline measurements we see that they are almost identical. This is due to the raw parameter count variation when changing the underlying architectures of our self-modeling networks. 

\begin{figure}[h!]
    \centering
    \includegraphics[width=\linewidth]{other_figures/vary_surrounding_layer_width_with_loss_with_baseline.png}
    \caption{Varying the layer width of the layers surrounding the target.}
    \label{fig:vary_surrounding_layer_width}
\end{figure}

\subsubsection{Modeling several layers at once}
 Finally, we explore the effect of allowing more than one layer to be the target of self-modeling. These networks have hidden layer structure given by $[2000, 1000, 1000, 500, 20]$. Initially, we added layers to the set of self-modeling targets starting the the earliest layer. Figure \ref{fig:target_multiple} shows a negligible effect on RLCT and loss when proceeding in this way. Given that the first layer was the largest, we repeated the experiment starting with only self-modeling the smallest and last layer and adding additional layers sequentially and show the analogous curves in Figure \ref{fig:reversed_target_multiple}. Here we see a clear elbow in the RLCT curve, indicating some threshold of self-modeled neurons over which a benefit is observed. It's worth noting that adding additional layers beyond the last three did not seem to yield an improved RLCT or generalization error.

\begin{figure}[t!]
    \centering
    \includegraphics[width=\linewidth]{other_figures/target_multiple_layers_with_loss_with_baseline.png}
    \caption{Allowing several layers to be the target of self-modeling.}
    \label{fig:target_multiple}
\end{figure}

\begin{figure}[t!]
    \centering
    \includegraphics[width=\linewidth]{other_figures/reversed_target_multiple_layers_with_loss_with_baseline.png}
    \caption{Allowing several target layers in the reverse order. We see a relationship between targeting large layers and improved generalization.}
    \label{fig:reversed_target_multiple}
\end{figure}
